# Supplementary material for: String-like Rearrangements Induce Mobility in Supercooled Liquids
Source: arXiv:2412.02923 ancillary file (2024-12-04)
Supplement: Supplementary file 1 [file SM.pdf]

# Supplementary Material for "Mobility Causes Mobility in Supercooled Liquids"

Rahul N. Chacko
*Department of Physics and Astronomy, University of Pennsylvania, Philadelphia, Pennsylvania 19104, USA*
(Dated: December 3, 2024)

## S1. NUMERICAL DETAILS

### A. Constants

The constant coefficients in the definition of the pair potential, alluded to in the main text, have values

$$c_0 = -28\tilde{r}_{\mathrm{cut}}^{-12}, \tag{1}$$
$$c_2 = 48\tilde{r}_{\mathrm{cut}}^{-14} \quad \text{and} \tag{2}$$
$$c_4 = -21\tilde{r}_{\mathrm{cut}}^{-16}. \tag{3}$$

The constants related to the size polydispersity of particles are

$$\sigma_{\min} \approx 0.7244461244, \tag{4}$$
$$\sigma_{\max} \approx 1.6138530488 \quad \text{and} \tag{5}$$
$$A \approx 1.3145271918, \tag{6}$$

where $A$ is the coefficient in the size distribution of particles, such that $P(\sigma) = A\sigma^{-3}$ for $\sigma \in [\sigma_{\min}, \sigma_{\max}]$.

Note that in many papers using this potential, including [1], each individual sample of $N = 10000$ particles has the particle sizes $\sigma$ rescaled such that the mean is exactly 1. In this paper (and in [2]), we do not do this rescaling, making our ensemble slightly different from that of other papers using this pair potential and polydispersity.

### B. Sample preparation

We prepare equilibrium configurations using a methodology developed by Ozawa for [3]. We conduct Monte Carlo simulations at constant temperature and volume, with two possible types of trial move. The first type of move, randomly selected with probability 0.8, is a trial displacement $(\Delta x, \Delta y)$ of a randomly selected particle, where both $\Delta x$ and $\Delta y$ are uniformly distributed in the interval $[-0.05, 0.05]$. The second type of move is a trial particle size swap $\sigma_i \mapsto \sigma_j$ and $\sigma_j \mapsto \sigma_i$. For a trial swap, a particle $i$ is randomly selected from the full set of particles, then a particle $j$ is randomly selected from the subset of particles satisfying $|\sigma_j - \sigma_i| < 0.2$. We initialise our configurations at infinite temperature before evolving the system at the target temperature until the potential energy reaches a steady state.

### C. Molecular dynamics

We conduct our molecular dynamics simulations in `LAMMPS` [4, 5] using the `NVE` thermostat, as appropriate for simulations in the microcanonical ensemble.

## S2. MERMIN-WAGNER FLUCTUATIONS

As a moderately-sized two-dimensional system, our system is subject to long-wavelength Mermin-Wagner fluctuations [6], as seen in Fig. S1. Following [7, 8], we can suppress the effect of these fluctuations on our results by replacing the raw displacement $\Delta\boldsymbol{r}_i^{\mathrm{raw}}$ of any particle $i$ with the "cage-relative" displacement

$$\Delta\boldsymbol{r}_i = \Delta\boldsymbol{r}_i^{\mathrm{raw}} - \frac{1}{|\mathcal{C}_i|}\sum_{j\in\mathcal{C}_i}\Delta\boldsymbol{r}_j^{\mathrm{raw}}, \tag{7}$$

where $\mathcal{C}_i$ is the set of all particles $j \neq i$ within some distance $\xi_{\mathrm{MW}}$ of particle $i$.

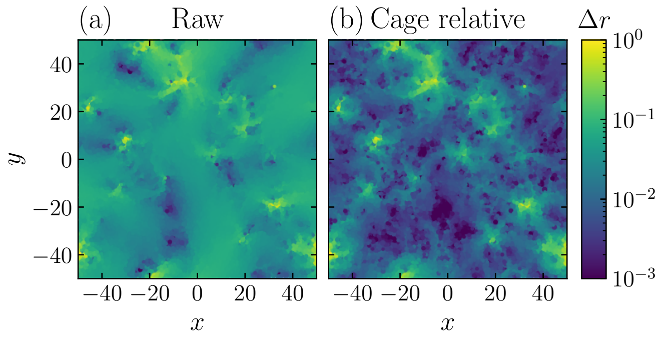


FIG. S1. Inherent state displacement of particles without (a) and with (b) accounting for Mermin-Wagner fluctuations through the use of cage-relative displacements (Eq. 7) with $\xi_{\mathrm{MW}} = 8.7$.

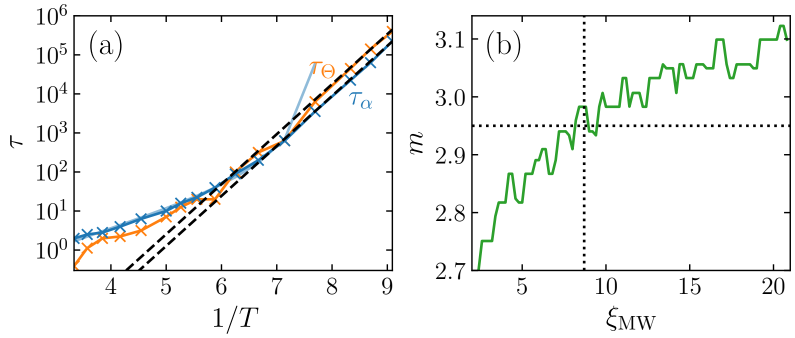


FIG. S2. (a): Relaxation times $\tau_\alpha$ (blue) and $\tau_\Theta$ (orange). The dashed lines show the ability of $\tau \sim \exp\left(2.95/T\right)$ to fit the low-temperature regime. (b): Energy scale $m$ for the exponential growth of $\tau_\alpha$ at low temperatures $T \le 0.140$ as a function of the length scale $\xi_{\mathrm{MW}}$ used when calculating cage-relative displacements. The dotted lines correspond to $\xi_{\mathrm{MW}} = 8.7$ and $m = 2.95$.

According to [9], the correct choice of $\xi_{\mathrm{MW}}$ is the dynamical length scale $\xi_{\mathrm{dyn}}$ [10]. However, for this system, we measure (see Supplementary Material of [1] for methodological details) large values of $\xi_{\mathrm{dyn}}$ at low temperatures, making this choice unsuitable for our system. For instance, we find $\xi_{\mathrm{dyn}} \approx 32$ at temperature $T = 0.110$, larger even than the typical size of Mermin-Wagner fluctuations that can be seen by eye in Fig. S1(a).

We therefore opt for a different approach to choosing $\xi_{\mathrm{MW}}$. Following [11], we choose a local structural indicator from which to extract a relaxation time without needing to account for Mermin-Wagner fluctuations. In our case, we extract the relaxation time $\tau_\Theta$ of the Tong and Tanaka $\Theta$ order parameter [12] (see [2] for methodological details) from the decay of the autocorrelation function

$$\mathrm{Corr}_\Theta\left(t\right) = \frac{\left\langle \Theta\left(0\right)\Theta\left(t\right)\right\rangle - \left\langle \Theta\left(0\right)^2\right\rangle}{\left\langle \Theta\left(0\right)^2\right\rangle - \left\langle \Theta\left(0\right)^2\right\rangle}. \tag{8}$$

Here, $\langle\cdot\rangle$ indicates an average over particles within one of ten bins of particle size $\sigma$, with bin boundaries spaced logarithmically in the interval $[\sigma_{\mathrm{min}}, \sigma_{\mathrm{max}}]$, accounting for the fact that particles of different size have different typical local structures. The resulting autocorrelation function $\mathrm{Corr}_\Theta\left(t\right)$ is then averaged over all particle bins and available configurations, and we obtain $\tau_\Theta$ from $t$ such that this quantity equals $1/e$. We find (Fig. S2(a)) that at low temperatures $T$, $\tau_\Theta \propto \exp\left(m_\Theta/T\right)$, where $m_\Theta \approx 2.95$.

We now calculate the bulk relaxation time $\tau_\alpha$. For an isotropic system, the self-intermediate scattering function [13] can be written

$$F_k\left(t\right) = \left\langle J_0\left(2\pi k \Delta r^{\mathrm{uq}}\right)\right\rangle, \tag{9}$$

where $J_0$ is the Bessel function of the first kind of order zero, $k$ is the wavenumber, $\Delta r^{\mathrm{uq}}$ is the magnitude of the unquenched (i.e., not inherent state) cage-relative displacement and $\langle\cdot\rangle$ denotes an average over all particles and

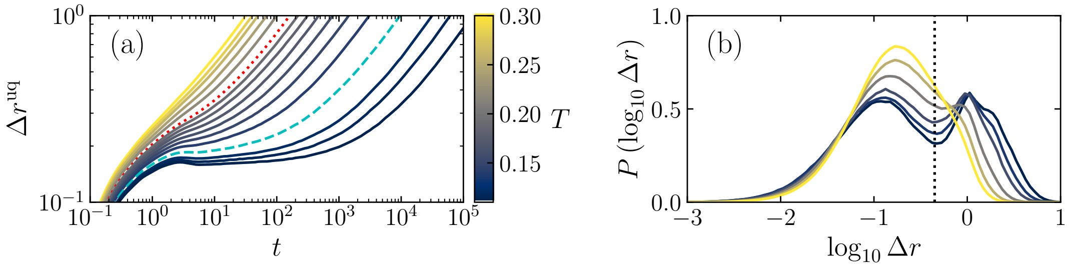


FIG. S3. (a): Root mean squared (unquenched) displacement of particles between times 0 and $t$. The red dotted line corresponds to $T = 0.200$ ($T_0$), while the cyan dashed line corresponds to $T = 0.130$ ($T_{\mathrm{MCT}}$). (b): Displacement (in the inherent state) distribution across a time interval of size $\tau_\alpha$ for temperatures $T = 0.110$, 0.115, 0.120, 0.130, 0.140 and 0.150 (curves darker to lighter). The vertical dotted line corresponds to the cage escape criterion $\Delta r^2 = 0.2$.

available configurations. We take $\tau_\alpha$ to be $t$ such that $F_1 = 1/e$, with $k = 1$ corresponding to the typical nearest-neighbour distance $r = 1$. Because $\Delta r_i$ will depend on our choice of $\xi_{\mathrm{MW}}$, we can calculate $\tau_\alpha$ as a function of $\xi_{\mathrm{MW}}$. Like $\tau_\Theta$, $\tau_\alpha$ exhibits Arrhenius behaviour $\tau_\alpha \propto \exp(m/T)$ at low temperatures. However, the energy scale $m$ depends on $\xi_{\mathrm{MW}}$ (Fig. S2(b)). We use this as a way of discriminating between different choices of $\xi_{\mathrm{MW}}$, choosing $\xi_{\mathrm{MW}} = 8.7$ so that $m = m_\Theta$.

## S3. TIME AND TEMPERATURE SCALES

From fitting $\log \tau_\alpha(T)$ (Fig. S2) in different temperature intervals and assuming that $\tau_\alpha$ is Arrhenius at low and high temperatures $T$ [11], we find

$$\log \tau_\alpha(T) = \begin{cases} -14.83 + 2.983/T & \text{if } T \leq 0.146, \\ -7.101 + 1.852/T & \text{if } 0.146 < T < 0.195, \\ -2.618 + 0.9758/T & \text{if } 0.195 \leq T. \end{cases} \tag{10}$$

If we define the onset temperature $T_0$ as the end of the high temperature Arrhenius regime, this gives us a value $T_0 \approx 0.2$ in line with that reported in [11].

A common approach to extracting the mode coupling theory temperature $T_{\mathrm{MCT}}$ is to fit the function $\tau_\alpha(T) = (T - T_{\mathrm{MCT}})^{-\gamma}$ to the data for $\tau_\alpha \in [\tau_0, 10^3\tau_0]$ [3, 11], where $\tau_0 = \tau_\alpha(T_0)$. However, this depends strongly on the precise choice of onset temperature $T_0$ and cutoff coefficient $10^3$. For $T_0 = 0.200$, this yields $T_{\mathrm{MCT}} = 0.115$. However, $T_0$ represents the onset of glassy behaviour, and different ways of characterising this exist. Examples include the onset of two-step relaxation in $F_k$ [14] or evidence of an inflection point between the ballistic and diffusive regimes (signalling the appearance of the caging plateau) in the root mean squared displacement (RMSD) of particles. As seen in Fig. S3(a), the latter would imply $T_0 \lesssim 0.300$, with the power-law divergence fit yielding $T_{\mathrm{MCT}} = 0.140$. Sastry *et al.* [15] suggest a characterisation of $T_{\mathrm{MCT}}$ independent of the chosen definition of $T_0$ as the temperature below which the displacement distribution $P(\log \Delta r(\tau_\alpha))$ becomes bimodal. As shown in Fig. S3(b), this definition yields $T_{\mathrm{MCT}} \approx 0.130$. Given the independence of this characterisation from arbitrary choices of $T_0$ or cutoff coefficient, we adopt $T_{\mathrm{MCT}} = 0.130$ as our mode coupling theory temperature.

Finally, from Fig. S3(a), we see that the ballistic regime lasts until $t \approx 0.3$, $t \approx 1$ corresponds to the crossover time between the ballistic regime and the caging plateau, while $t \approx 3$ marks the start of the caging plateau.

## S4. LONG TRAJECTORY

In Fig. S4, we show an extended version of the trajectory shown in Fig. 3(a) in the main text, indicating via coloured squares a few examples of regions that contain many rearrangement events over time. We see that the tendency for particles directly involved in one microstring to subsequently participate directly in a different microstring is general and can persist over long intervals of time.

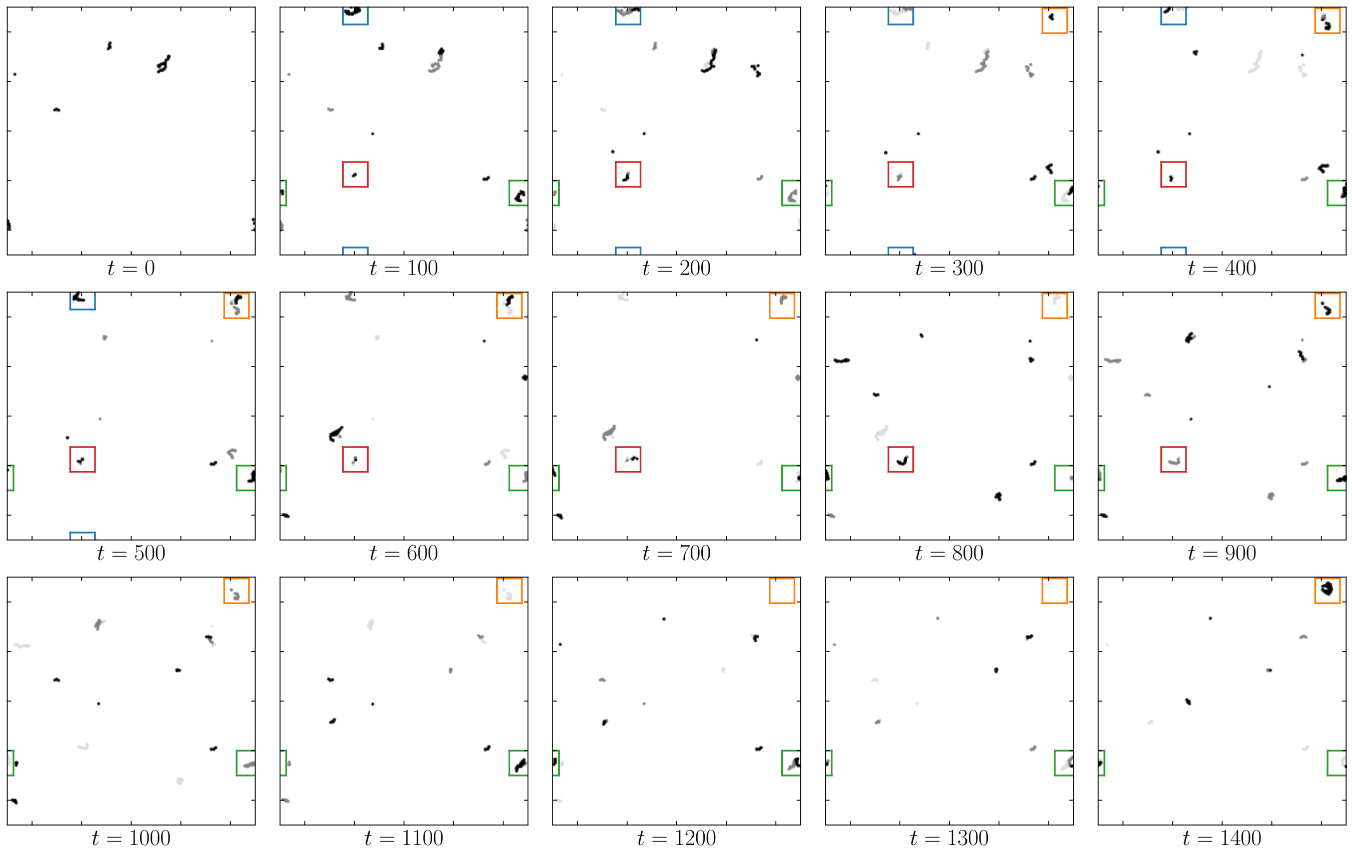


FIG. S4. Extended version of the trajectory shown in Fig. 3(a) of the main text. The black points are particles that escape their cage between the snapshot they appear in and time $\Delta t = 100$ later. The grey points in a snapshot are copies of the black points from the previous snapshot. The light points correspond to grey points from the previous snapshot. The region shown in Fig. 3(a) is within the blue square.

## S5. TEMPERATURE DEPENDENCE

In the main text, we show how the results of our analysis changes as the time available for avalanching rearrangements increases for the single temperature $T = 0.110$. In Fig. S5, we instead fix a short $\Delta t$ and show how the results of our analysis vary with temperature. Broadly, we find that increasing the temperature has a similar effect to increasing the time scale $\Delta t$.

## S6. HOP CRITERION DEPENDENCE

In the main text, we impose a fairly severe criterion for what counts as a hop. Ultimately, however, it is known that the length scales separating cages vary greatly [16], and so no single threshold can capture every hopping event, in which a particle changes its local structural environment, while rejecting smaller, reversible displacements. It is therefore worth seeing how robust our analysis is to varying the threshold size. In Fig. S6, we show the result of halving our displacement criterion for hopping to $\Delta r^2 > 0.05$.

For the trajectory shown in Fig. S6(a), we see larger clusters of displacement. Notably, in the second row, we see a microstring which encapsulates an entire Eshelby quadrupole [17], showing that this reduced hop criterion counts much of the elastic displacement quadrupole [1, 17, 18]. Indeed, making equivalent plots of Fig. S6(a) for other rearrangement events in the long trajectory of Fig. S4 (not shown) yields similar behaviour, including counting much of the displacement quadrupole as a cage hop. This is consistent with the idea that the elastic signature of rearrangements reported by this author in previous work [1] in fact relates to the structure of individual microstrings themselves, rather than to the propagation of mobility between distinct rearrangement events, separated in space and time.

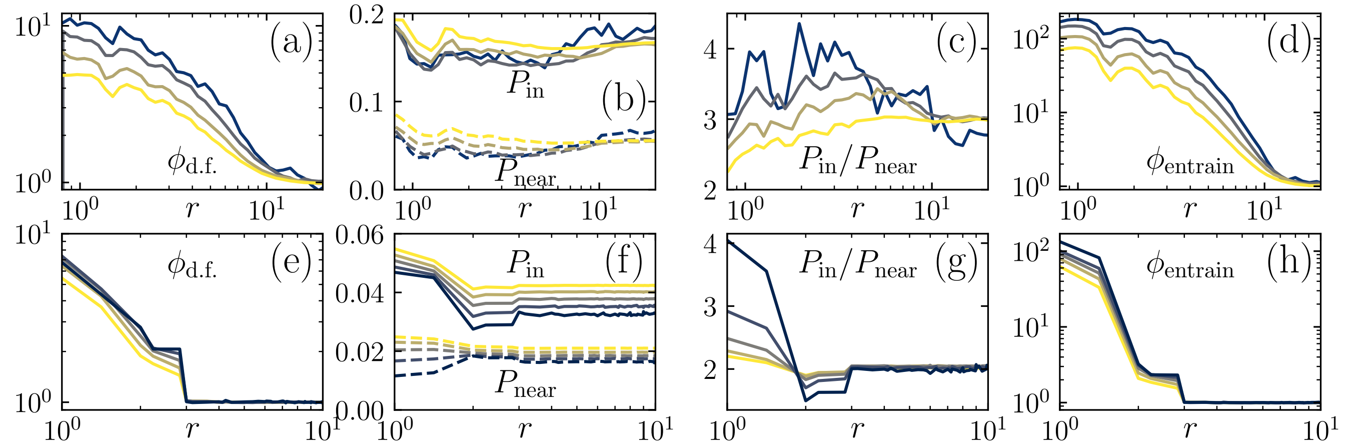


FIG. S5. (a)–(d): Temperature-dependent versions of Figs. 2(b)–2(e) from the main text, with $\Delta t = 3$ fixed and $T = 0.105$, 0.120, 0.140 and 0.160 (darker to lighter). (e)–(h): Temperature-dependent versions of Figs. 4(a)–4(d) from the End Matter, with $\Delta t = 10^{-1}$ fixed and $T = 0.30$, 0.35, 0.40, 0.45 and 0.50.

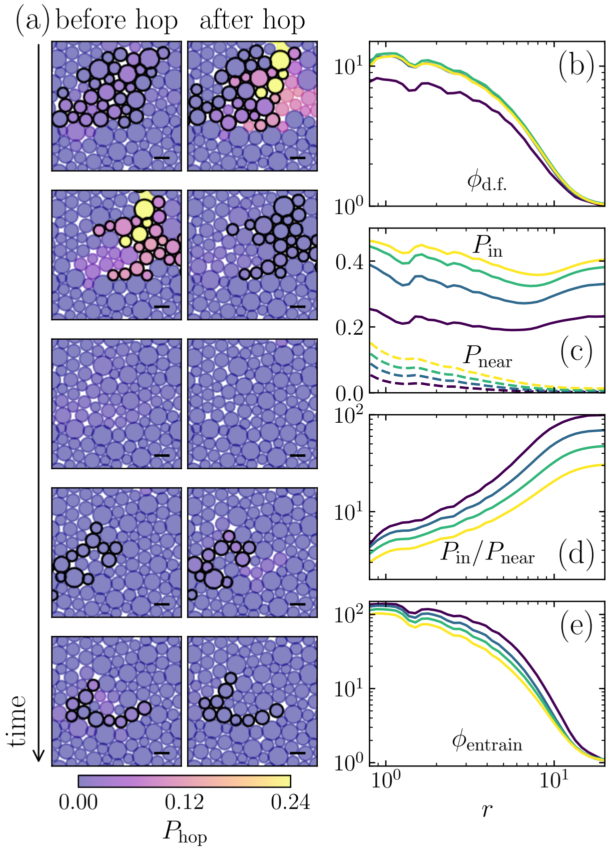


FIG. S6. Fig. 2 of the main text, reproduced with a hop criterion reduced to $\Delta r^2 > 0.05$.

With respect to our analysis, Figs. 2(b)–2(e), we obtain corresponding results (Figs. S6(a)–S6(e)) that are qualitatively unchanged except that $\Delta t = 3$ is no longer short enough to fully suppress the $r$-dependence of $P_{\text{near}}$. The trend of $P_{\text{near}}$ flattening as $\Delta t$ is decreased is nonetheless clear.

[1] R. N. Chacko, F. P. Landes, G. Biroli, O. Dauchot, A. J. Liu, and D. R. Reichman, Phys. Rev. Lett. **127**, 048002 (2021).
[2] R. N. Chacko, F. P. Landes, G. Biroli, O. Dauchot, A. J. Liu, and D. R. Reichman, Phys. Rev. X **14**, 031012 (2024).
[3] L. Berthier, P. Charbonneau, A. Ninarello, M. Ozawa, and S. Yaida, Nat Commun **10**, 1508 (2019).
[4] S. Plimpton, Journal of Computational Physics **117**, 1 (1995).
[5] A. P. Thompson, H. M. Aktulga, R. Berger, D. S. Bolintineanu, W. M. Brown, P. S. Crozier, P. J. in 't Veld, A. Kohlmeyer, S. G. Moore, T. D. Nguyen, R. Shan, M. J. Stevens, J. Tranchida, C. Trott, and S. J. Plimpton, Computer Physics Communications **271**, 108171 (2022).
[6] E. Flenner and G. Szamel, Nat Commun **6**, 7392 (2015).
[7] S. Vivek, C. P. Kelleher, P. M. Chaikin, and E. R. Weeks, Proc. Natl. Acad. Sci. U.S.A. **114**, 1850 (2017).
[8] B. Illing, S. Fritschi, H. Kaiser, C. L. Klix, G. Maret, and P. Keim, Proc. Natl. Acad. Sci. U.S.A. **114**, 1856 (2017).
[9] R. Das, I. Tah, and S. Karmakar, The Journal of Chemical Physics **149**, 024501 (2018).
[10] N. Lačević, F. W. Starr, T. B. Schrøder, and S. C. Glotzer, The Journal of Chemical Physics **119**, 7372 (2003).
[11] C. Scalliet, B. Guiselin, and L. Berthier, Phys. Rev. X **12**, 041028 (2022).
[12] H. Tong and H. Tanaka, Phys. Rev. X **8**, 011041 (2018).
[13] O. Dauchot, G. Marty, and G. Biroli, Phys. Rev. Lett. **95**, 265701 (2005).
[14] D. Coslovich, L. Galliano, and L. Costigliola, Freezing, melting and the onset of glassiness in binary mixtures (2024), arXiv:2406.04921.
[15] S. Sastry, P. G. Debenedetti, and F. H. Stillinger, Nature **393**, 554 (1998).
[16] A. S. Keys, L. O. Hedges, J. P. Garrahan, S. C. Glotzer, and D. Chandler, Phys. Rev. X **1**, 021013 (2011).
[17] G. Picard, A. Ajdari, F. Lequeux, and L. Bocquet, Eur. Phys. J. E **15**, 371 (2004).
[18] J. D. Eshelby, Proc. R. Soc. Lond. A **241**, 376 (1957).
